# Supplementary material for: Optimum Methods for Quasi-Orthographic Surface Imaging
Source: arXiv:2305.08121 source file (2023-05-14)
Supplement: Supplementary file 1 [file AppendixA.tex]

% Appendix Template

\chapter{Appendix A} % Main appendix title

\label{AppendixX} % Change X to a consecutive letter; for referencing this appendix elsewhere, use \ref{AppendixX}

\lhead{Appendix X. \emph{Appendix Title Here}} % Change X to a consecutive letter; this is for the header on each page - perhaps a shortened title

Write your Appendix content here.
